# Supplementary material for: Capturing Conditional Dependence via Auto-regressive Diffusion Models
Source: arXiv:2504.21314 source file (2025-04-30)
Supplement: Supplementary file 1 [file 0X3_causal_example.tex]

\section{Causal Examples}
In this section, we consider a special setting of auto-regressive diffusion models.
Suppose we expect to generate a sample $(\rvx_1,\rvx_2)$ from a joint distribution $p_*(\vx_1,\vx_2)$ where $\vx_1,\vx_2\in \R^d$ and 
\begin{equation*}
    p_{*,2|1}(\vx_2|\vx_1) \propto \exp\left(-\frac{\|\vx_2- \vx_1\|^2}{2\sigma^2}\right).
\end{equation*}
Such a condition can also be presented from a random variable perspective, i.e.,
\begin{equation*}
    \rvx_2 = f(\rvx_1) + \sigma\cdot \xi\quad \text{where}\quad \xi\sim \mathcal{N}(\vzero,\mI)
\end{equation*}
and $f\colon \R^d\rightarrow \R^d$ is an one-one map.
% sharp mix small variance large variance
\begin{lemma}
    TBC
\end{lemma}
\begin{proof}
    We consider the case by setting $k = 1$ in Lemma~\ref{lem:condi_rtk_error_eachk}.
    Then, with the same notation, Eq.~\ref{ineq:kl_error_eachk} can be written as
    \begin{equation*}
        \begin{aligned}
            &\KL{p_{*,k+1|[1:k]}(\cdot|\rvx_{[1:k]})}{p^\gets_{*,k+1|[1:k]}(\cdot|\rvx_{[1:k]})}\\
            &  = \KL{\tilde{q}_T}{q^\gets_T} \le \KL{\tilde{q}_{t_{R-1}}}{q^\gets_{t_{R-1}}}+ \E_{\tilde{\rvy}\sim \tilde{q}_{t_{R-1}}}\left[\KL{\tilde{q}_{t_R|t_{R-1}}(\cdot|\tilde{\rvy})}{q^\gets_{t_R|t_{R-1}}(\cdot|\tilde{\rvy})}\right]\\
            & \le \KL{\tilde{q}_0}{q^\gets_0} + \underbrace{ \sum_{r=0}^{R-1} \E_{\tilde{\rvy}\sim \tilde{q}_{t_r}}\left[\KL{\tilde{q}_{t_{r+1}|t_r}(\cdot|\tilde{\rvy})}{q^\gets_{t_{r+1}|t_r}(\cdot|\tilde{\rvy})}\right]}_{\text{reverse transition error}}.
            \end{aligned}
    \end{equation*} 
     where the first inequality follows from the chain rule, i.e., Lemma~\ref{lem:tv_chain_rule}, of KL divergence, and the second one follows from the recursive manner. 
    Besides, we have $\tilde{q}_0^\gets = \varphi_1$ which denotes the density function of $\mathcal{N}(\vzero, \mI)$.

    \paragraph{Initialization Error.} We first consider to upper bound $\TVD{q_T}{\varphi_1}$. 
    Due to Lemma~\ref{lem:initialization_error}, we have
    \begin{equation*}
        \begin{aligned}
            & \KL{\tilde{q}_0}{q_0^\gets} = \KL{q_T}{\varphi_1}\le e^{-2T}\cdot \KL{p^\to_{k+1|[1:k], 0}(\cdot|\vx_{1:k})}{\varphi_1}\\
            & \le e^{-2T}\cdot \left(2Ld_{k+1} + \E_{p_{*,k+1|[1:k]}(\cdot|\vx_{[1:k]})}\left[\|\rvy\|^2\right] \right).
        \end{aligned}
    \end{equation*}

    \paragraph{Reverse Transition Error.}
    According to Lemma~\ref{lem:kl_diff_close}, the reverse transition error can be relaxed as
    
\end{proof}

\begin{lemma}
    \label{lem:kl_diff_close}
    TBC
\end{lemma}
\begin{proof}
    According to the definition of the forward process, i.e., Eq.~\ref{sde:ideal_condi_forward}, for $k=1$ and given $\vx_1$, there is $q_0(\cdot) = p_{*,2|1}(\cdot|\vx_1)$ whose closed form is 
    \begin{equation*}
        q_0(\vy) = \tilde{q}_T(\vy)\propto \exp\left(-\frac{\|\vy - f(\vx_1)\|^2}{2\sigma^2}\right).
    \end{equation*}
    With the OU forward process for $\rvy_t$, i.e., Eq.~\ref{sde:ideal_condi_forward}, we have
    \begin{equation*}
        \rvy_t = e^{-t}\rvy_0 + \sqrt{1-e^{-2t}}\cdot \xi\quad \xi\sim \mathcal{N}(\vzero,\mI).
    \end{equation*}
    Since the convolution of two Gaussian distributions is still a Gaussian distribution, the expectation and variance can be calculated by
    \begin{equation*}
        \begin{aligned}
            & \E[\rvy_t] = e^{-t}\E[\rvy_0] + \sqrt{1-e^{-2t}}\E[\xi] = e^{-t}f(\vx_1)\\
            & \Var[\rvy_t] = e^{-2t}\cdot \Var[\rvy_0] + (1-e^{-2t})\cdot\Var[\xi] = \left[e^{-2t}\sigma^2 + (1-e^{-2t})\right]\mI,
        \end{aligned}
    \end{equation*}
    which means
    \begin{equation}
        \label{ineq:causal_q_t_close_form}
        q_t(\vy)\propto \exp\left(-\frac{\|\vy - e^{-t}f(\vx_1)\|^2}{2\left[e^{-2t}\sigma^2 + (1-e^{-2t})\right]}\right).
    \end{equation}
    According to Bayes Theorem, we have
    \begin{equation*}
        \begin{aligned}
            q_{r\eta|(r+1)\eta}(\vy^\prime|\vy)&  = \frac{q_{(r+1)\eta|r\eta}(\vy|\vy^\prime)\cdot q_{r\eta}(\vy^\prime)}{q_{(r+1)\eta}(\vy)}\\
            & = q^{-1}_{(r+1)\eta}(\vy)\cdot Z_{(r+1)\eta|r\eta}^{-1}\cdot \exp\left(-\frac{\left\|\vy - e^{-\eta}\vy^\prime\right\|^2}{2(1-e^{-2\eta})}\right)\cdot Z^{-1}_{r\eta}\cdot \exp\left(-\frac{\|\vy - e^{-t}f(\vx_1)\|^2}{2\left[e^{-2t}\sigma^2 + (1-e^{-2t})\right]}\right)\\
            & \propto \exp\left(-\frac{\left\|\vy - e^{-\eta}\vy^\prime\right\|^2}{2(1-e^{-2\eta})}-\frac{\|\vy - e^{-t}f(\vx_1)\|^2}{2\left[e^{-2t}\sigma^2 + (1-e^{-2t})\right]}\right)
        \end{aligned}
    \end{equation*}
    where the second inequality follows from the transition kernel of the OU process and Eq.~\ref{ineq:causal_q_t_close_form}.
    Then, we simplify its energy function in the following:
    \begin{equation*}
        \begin{aligned}
            & -\ln q_{r\eta|(r+1)\eta}(\vy^\prime|\vy)  = \frac{\left\|\vy - e^{-\eta}\vy^\prime\right\|^2}{2(1-e^{-2\eta})} + \frac{\|\vy - e^{-t}f(\vx_1)\|^2}{2\left[e^{-2t}\sigma^2 + (1-e^{-2t})\right]} +C\\
            & = \frac{\|\vy^\prime\|^2}{2(e^{2\eta}-1)}  - \left<\vy^\prime, \frac{e^{\eta}\cdot \vy}{e^{2\eta}-1}\right> + \frac{e^{2\eta}\|\vy\|^2}{2(e^{2\eta}-1)} + C\\
            &\quad + \frac{\|\vy^\prime\|^2}{2\left[e^{-2r\eta}\sigma^2 + (1-e^{-2r\eta})\right]} -\left<\vy^\prime, \frac{e^{-r\eta}\cdot f(\vx_1)}{e^{-2r\eta}\sigma^2 + (1-e^{-2r\eta})}\right> + \frac{e^{-2r\eta}\left\|f(\vx_1)\right\|^2}{2\left[e^{-2r\eta}\sigma^2 + (1-e^{-2r\eta})\right]}
        \end{aligned}
    \end{equation*}
    By supposing
    \begin{equation*}
        C^\prime(\vy, \vx_1) \coloneqq \frac{e^{2\eta}\|\vy\|^2}{2(e^{2\eta}-1)} + \frac{e^{-2r\eta}\left\|f(\vx_1)\right\|^2}{2\left[e^{-2r\eta}\sigma^2 + (1-e^{-2r\eta})\right]} + C,
    \end{equation*}
    we have
    \begin{equation*}
        \begin{aligned}
            & -\ln q_{r\eta|(r+1)\eta}(\vy^\prime|\vy) = \frac{\|\vy^\prime\|^2}{2}\cdot \left[\frac{1}{e^{2\eta} - 1} + \frac{1}{e^{-2\eta}\sigma^2+1 - e^{-2r\eta}}\right] -\left<\vy^\prime, \frac{e^{\eta}\cdot \vy}{e^{2r\eta}-1} + \frac{e^{-r\eta}\cdot f(\vx_1)}{e^{-2r\eta}\sigma^2 + (1-e^{-2r\eta})} \right> + C^\prime(\vy,\vx_1)\\
            & = \left\|\sqrt{\frac{1}{2}\cdot\left(\frac{1}{e^{2\eta} - 1} + \frac{1}{e^{-2r\eta}\sigma^2+1 - e^{-2r\eta}}\right)\cdot \vy^\prime} - \frac{\frac{e^{\eta}\cdot \vy}{e^{2\eta}-1} + \frac{e^{-r\eta}\cdot f(\vx_1)}{e^{-2r\eta}\sigma^2 + (1-e^{-2r\eta})} }{2\cdot \sqrt{\frac{1}{2}\cdot\left(\frac{1}{e^{2\eta} - 1} + \frac{1}{e^{-2r\eta}\sigma^2+1 - e^{-2r\eta}}\right)}}\right\|^2\\
            & \quad - \left\|\frac{\frac{e^{\eta}\cdot \vy}{e^{2\eta}-1} + \frac{e^{-r\eta}\cdot f(\vx_1)}{e^{-2r\eta}\sigma^2 + (1-e^{-2r\eta})} }{2\cdot \sqrt{\frac{1}{2}\cdot\left(\frac{1}{e^{2\eta} - 1} + \frac{1}{e^{-2r\eta}\sigma^2+1 - e^{-2r\eta}}\right)}}\right\|^2 + C^\prime(\vy,\vx_1).
        \end{aligned}
    \end{equation*}
    Considering the last two terms of the previous equation are constants, that means we have
    \begin{equation*}
        q_{r\eta|(r+1)\eta}(\vy^\prime|\vy)\propto \exp\left[-\frac{\left\|\vy^\prime - \frac{\frac{e^{\eta}\cdot \vy}{e^{2\eta}-1} + \frac{e^{-r\eta}\cdot f(\vx_1)}{e^{-2r\eta}\sigma^2 + (1-e^{-2r\eta})} }{\frac{1}{e^{2\eta} - 1} + \frac{1}{e^{-2\eta}\sigma^2+1 - e^{-2r\eta}}}\right\|^2}{2\cdot \left(\frac{1}{\frac{1}{e^{2\eta} - 1} + \frac{1}{e^{-2r\eta}\sigma^2+1 - e^{-2r\eta}}}\right)}\right]
    \end{equation*}
    which is a Gaussian-type distribution with
    \begin{equation*}
        \vmu_1 = \frac{\frac{e^{\eta}\cdot \vy}{e^{2\eta}-1} + \frac{e^{-r\eta}\cdot f(\vx_1)}{e^{-2r\eta}\sigma^2 + (1-e^{-2r\eta})} }{\frac{1}{e^{2\eta} - 1} + \frac{1}{e^{-2r\eta}\sigma^2+1 - e^{-2r\eta}}}\quad \text{and}\quad \sigma_1^2 = \frac{1}{\frac{1}{e^{2\eta} - 1} + \frac{1}{e^{-2r\eta}\sigma^2+1 - e^{-2r\eta}}}.
    \end{equation*}
    With a slightly different DDPM-type update of the reverse OU process as follows:
    \begin{equation*}
        \rvy^\gets_{(R-r)\eta} = e^\eta\rvy^\gets_{[R-(r+1)]\eta}+2\cdot (e^\eta - 1)\vs_{\vtheta, (r+1)\eta} + \sqrt{\frac{(1-\eta^{1.5})^{-1}}{\frac{1}{e^{2\eta} - 1} + \frac{1}{e^{-2r\eta}u+1 - e^{-2r\eta}}}}\cdot\xi\quad \text{where}\quad \xi\sim\mathcal{N}(\vzero,\mI),
    \end{equation*}
    we have the following conditional probability, i.e.,
    \begin{equation*}
        q^\gets_{(R-r)\eta|[R-(r+1)]\eta}(\vy^\prime|\vy)\propto \exp\left[-\frac{\left\|\vy^\prime - \left(e^\eta\cdot  \vy + 2(e^\eta-1)\cdot \vs_{\vtheta, (r+1)\eta}\right)\right\|^2}{2\left(\frac{(1-\eta^{1.5})^{-1}}{\frac{1}{e^{2\eta} - 1} + \frac{1}{e^{-2r\eta}u+1 - e^{-2r\eta}}}\right)}\right]
    \end{equation*}
    which is also a Gaussian-type distribution with
    \begin{equation*}
        \vmu_2 = e^\eta\cdot  \vy + 2(e^\eta-1)\cdot \vs_{\vtheta, (r+1)\eta} \quad \text{and}\quad \sigma_2^2 = \frac{1}{\frac{1}{e^{2\eta} - 1} + \frac{1}{e^{-2r\eta}u+1 - e^{-2r\eta}}}\cdot (1-\eta^{1.5})^{-1}.
    \end{equation*}
    Considering the KL divergence between $q_{r\eta|(r+1)\eta}(\cdot|\vy) = \tilde{q}_{(R-r)\eta|[R-(r+1)]\eta}(\cdot|\vy)$ and $q^\gets_{(R-r)\eta|[R-(r+1)]\eta}(\cdot|\vy)$, we have
    \begin{equation}
        \label{eq:kl_div_two_gau}
        \KL{q^\gets_{(R-r)\eta|[R-(r+1)]\eta}(\cdot|\vy)}{\tilde{q}_{(R-r)\eta|[R-(r+1)]\eta}(\cdot|\vy)} = \frac{d}{2}\cdot \underbrace{\left(\ln \frac{\sigma_1^2}{\sigma_2^2} + \frac{\sigma_2^2}{\sigma_1^2} -1\right)}_{\text{Term 1}} + \frac{1}{2}\cdot \underbrace{\frac{\|\vmu_1 - \vmu_2\|^2}{\sigma_1^2}}_{\text{Term 2}}.
    \end{equation}
    For Term 1, we have
    \begin{equation*}
        \begin{aligned}
            &\text{Term 1} = \ln\left(1-\frac{\sigma_2^2-\sigma_1^2}{\sigma_2^2}\right) + \frac{\sigma_2^2}{\sigma_1^2} - 1 \le  \left|1 - \frac{\sigma_1^2}{\sigma_2^2}\right|^2\le \eta^3
        \end{aligned}
    \end{equation*}
    where the last inequality follows from
    \begin{equation*}
        \frac{\sigma_1^2}{\sigma_2^2} =(1-\eta^{1.5})\cdot  \frac{\frac{1}{e^{2\eta} - 1} + \frac{1}{e^{-2r\eta}u+1 - e^{-2r\eta}}}{\frac{1}{e^{2\eta} - 1} + \frac{1}{e^{-2r\eta}\sigma^2+1 - e^{-2r\eta}}}\le 
    \end{equation*}
    
\textcolor{red}{\hrule}
    
    where 
    \begin{equation*}
        \Delta = \frac{e^{2\eta}-1}{e^{-2r\eta}\sigma^2+1 - e^{-2r\eta}}
    \end{equation*}
   Then, we have
    \begin{equation*}
        \text{Term 1}\le \frac{\Delta^2}{2(1+\Delta)}\le \frac{\Delta^2}{2}\le 8\eta^2\cdot \max\left\{1,\frac{1-\sigma^2}{\sigma^2}\right\}^2 
    \end{equation*}
    where the last inequality follows from 
    \begin{equation*}
        e^{2\eta} - 1\le 4\eta\quad \text{when}\quad \eta\le 1/2,
    \end{equation*}
    and Lemma~\ref{}.

    For Term 2, Eq.~\ref{ineq:causal_q_t_close_form} implies that
    \begin{equation*}
        \grad\ln q_{r\eta}(\vy) = -\frac{\vy - e^{-r\eta}\cdot f_1(\vx_1) }{e^{-2r\eta}\sigma^2 + 1 - e^{-2r\eta}} \quad \Leftrightarrow\quad \grad\ln q_{r\eta}(\vy) + \frac{\vy}{e^{-2r\eta}\sigma^2 + 1 -e^{-2r\eta}} = \frac{e^{-r\eta}\cdot f(\vx_1)}{e^{-2r\eta}\sigma^2 + 1 - e^{-2r\eta}},
    \end{equation*}
    which means
    \begin{equation*}
        \begin{aligned}
            &\vmu_1 = e^\eta\cdot \vy\cdot \frac{1}{\left(\frac{1}{e^{2\eta} - 1} + \frac{1}{e^{-2r\eta}\sigma^2+1 - e^{-2r\eta}}\right)\cdot (e^{2\eta}-1)} + \frac{ \frac{e^{-r\eta}\cdot f(\vx_1)}{e^{-2r\eta}\sigma^2 + (1-e^{-2r\eta})} }{\frac{1}{e^{2\eta} - 1} + \frac{1}{e^{-2r\eta}\sigma^2+1 - e^{-2r\eta}}}\\
            & = e^\eta\cdot \vy\cdot \frac{1}{\left(\frac{1}{e^{2\eta} - 1} + \frac{1}{e^{-2r\eta}\sigma^2+1 - e^{-2r\eta}}\right)\cdot (e^{2\eta}-1)} + \frac{\grad\ln q_{r\eta}(\vy) + \frac{\vy}{e^{-2r\eta}\sigma^2 + 1 -e^{-2r\eta}}}{\frac{1}{e^{2\eta} - 1} + \frac{1}{e^{-2r\eta}\sigma^2+1 - e^{-2r\eta}}}\\
            & = e^\eta\cdot \left[\frac{1}{1+\Delta}+ \frac{e^{-\eta}}{1+1/\Delta}\right]\cdot\vy + \left(\frac{1}{\frac{1}{e^{2\eta} - 1} + \frac{1}{e^{-2r\eta}\sigma^2+1 - e^{-2r\eta}}}\right)\cdot \grad\ln q_{r\eta}(\vy).
        \end{aligned}
    \end{equation*}
    Therefore, we have
    \begin{equation*}
        \begin{aligned}
            \text{Term 2} = \frac{1}{TBC}
        \end{aligned}
    \end{equation*}

\end{proof}
